# Supplementary material for: Ground-state Pulsed Cavity Electro-optics for Microwave-to-optical Conversion
Source: arXiv:2010.11392 ancillary file (2020-10-22)
Supplement: Supplementary file 1 [file EO_Converter_ground_state_SI_10212020.pdf]

# Supplementary Information for "Ground-state Pulsed Cavity Electro-optics for Microwave-optical Conversion"

Wei Fu,[1,*] Mingrui Xu,[1,*] Xianwen Liu,[1] Chang-Ling Zou,[1] Changchun Zhong,[2] Xu Han,[1] Mohan Shen,[1] Yuntao Xu,[1] Risheng Cheng,[1] Sihao Wang,[1] Liang Jiang,[2,3] and Hong X. Tang[1,3,†]

[1] *Department of Electrical Engineering, Yale University, New Haven, Connecticut 06520, USA*
[2] *Pritzker School of Molecular Engineering, University of Chicago, Illinois 60637, USA*
[3] *Yale Quantum Institute, Yale University, New Haven, Connecticut 06520, USA*

* These authors contributed equally to this work.
† hong.tang@yale.edu

## NOTE 1. DEVICE DESIGN AND FABRICATION

For the photonic chip, approximately 1 $\mu$m single-crystalline AlN is grown on c-plane sapphire by metalorganic chemical vapor deposition (MOCVD). The double-rings and bus optical waveguides are defined with negative FOx-16 resist by an 100 kV electron-beam lithography (EBL) system (Raith EBPG 5000+). Gold is deposited to mitigate charging effect and removed after the EBL process. Then, the pattern is transferred to AlN with an optimized Cl2/BCl3/Ar-based inductively coupled plasma (ICP) etching. Finally, the wafer is embedded in 1.5-$\mu$m silicon dioxide by plasma-enhanced chemical vapor deposition (PECVD) and is cleaved for side-coupling and fiber-gluing.

The superconducting resonator is fabricated from a 50 nm-thick niobium nitride (NbN) film deposited on a sapphire substrate via atomic layer deposition. The pattern is defined by one single ebeam lithography step using hydrogen silsesquioxane (HSQ) resist, followed by chlorine dry etching. The remaining HSQ mask is removed using diluted buffered oxide etch.

The ground-signal-ground capacitor of the microwave resonator is designed to provide out-of-plane electric field, which couples to the transverse electrical optical modes via electro-optical coefficient $r_{13}$ of AlN. The overlap between the electrical field of the microwave mode and the optical microring is simulated in COMSOL. By assuming homogeneous electrical field generated by the superconducting resonator in the photonic microring, as well as a Pockel's coefficient $r_{13} = 1$ pm/V, from the simulation we can estimate the vacuum eletro-optical coupling rate $g_\mathrm{o}$ to be around 300 Hz, when the vacuum gap between the surfaces of the superconducting resonator and the oxide of the photonic chip are 2 $\mu$m. Larger gap will result in less coupling rate. When the gap is 4 $\mu$m, the coupling rate becomes 70% of the value corresponding to a 2$\mu$m-gap. When the gap is 10 $\mu$m, the coupling rate drops to 30% of that value. The in-plane misalignment within 2 $\mu$m does not significantly compromise the coupling $g_\mathrm{o}$. Based on experimentally inferred $g_\mathrm{o}$, the gap between the superconducting chip and the photonic chip is estimated to be around 14 $\mu$m.

The details of the design to enable superconducting resonant frequency tunability can be found in Ref. [S2]. On the resonator, hole structures are patterned in the high-kinetic inductance wire. By applying a perpendicular external magnetic field, the kinetic inductance can be modified by the induced screening supercurrent circulating the holes, thus the resonant frequency can be wirelessly shifted.

## NOTE 2. DEVICE BASIC CHARACTERISTICS

Shown in Table S1 are basic device characteristics when applying a -11.4 dBm pulsed optical drive during the period when the drive is on. Corresponding conversion efficiency is characetrized to be $3.3 \times 10^{-6}$. Subscript $a$, $b$, and $c$ correspond to the optical drive, optical signal, and microwave modes, respectively. When thermalized at 40 mK without any optical drive, the superconducting resonator has an intrinsic quality factor $Q_\mathrm{in}$ of 6000. $Q_\mathrm{in}$ varies with different optical drive because of the changes in ambient temperature as well as quasi-particle generation (Fig. 4). All the other parameters are relatively constant and the system can be treated as a steady state when the optical drive is shined on the device. The extraction ratio of the microwave mode as well as the optical mode, defined as the external coupling rate devided by the total coupling rate, are around 7% and 44%, respectively.

TABLE S1. device characteristics.

| $f_\mathrm{c}$ | $\kappa_\mathrm{c,ex}/2\pi$ | $\kappa_\mathrm{c,in}/2\pi$ | $\lambda_\mathrm{a}$ | $\kappa_\mathrm{a,ex}/2\pi$ | $\kappa_\mathrm{a,in}/2\pi$ | $\kappa_\mathrm{b,ex}/2\pi$ | $\kappa_\mathrm{b,in}/2\pi$ | $g_\mathrm{o}/2\pi$ |
|---|---|---|---|---|---|---|---|---|
| 6.412 GHz | 100 kHz | 1.36 MHz | 1554.9 nm | 37 MHz | 92 MHz | 61 MHz | 79 MHz | 42 Hz |

The peak conversion efficiency is linked to the device characteristics through equation:

$$\eta_{peak} = \frac{\kappa_\mathrm{c,ex}}{\kappa_\mathrm{c}} \frac{\kappa_\mathrm{b,ex}}{\kappa_\mathrm{b}} \frac{4C}{(1+C)^2}, \tag{S1}$$

where

$$C = \frac{4 g_\mathrm{o}^2 n_\mathrm{drive}^2}{\kappa_\mathrm{a}\kappa_\mathrm{b}} = \frac{4 g_\mathrm{o}^2}{\kappa_\mathrm{a}\kappa_\mathrm{b}} \frac{P_\mathrm{drive}\kappa_\mathrm{a,ex}}{(\kappa_\mathrm{a}/2)^2}. \tag{S2}$$

Detailed derivation of these equations can be found in reference [1]. Here $C$ is cooperativity, $\kappa_\mathrm{a} = \kappa_\mathrm{a,in} + \kappa_\mathrm{a,ex}$, $\kappa_\mathrm{b} = \kappa_\mathrm{b,in} + \kappa_\mathrm{b,ex}$ and $\kappa_\mathrm{c} = \kappa_\mathrm{c,in} + \kappa_\mathrm{c,ex}$ are the total coupling rates of the modes. $g_\mathrm{o}$ is the vacuum eletro-optical coupling coefficient. $P_\mathrm{drive}$ is the optical drive power in the waveguide. In using equation S1, we assume the detuning between the microwave resonant frequency and the optical modes splitting, as well as the detuning between the

optical drive frequency and pump mode frequency are negligible. During the measurement, the detuning between the microwave resonant frequency and the optical mode splitting is within 10 MHz, well below the optical signal mode decay rate $\kappa_b$. The optical drive was locked within 10% of the optical pump mode total decay rate from the pump mode resonant frequency. Given such conditions, we can use equation S1, device parameters listed in table S1 and experimentally characterized conversion efficiency with -11.4 dBm optical drive to estimate the vacuum electro-optical coupling coefficient $g_o$, which is found to be $2\pi \times 42$ Hz. Considering that the experimental condition does not perfectly match the assumptions such as zero detuning, the actual electro-optical coupling coefficient could be slightly larger.

## NOTE 3. MEASUREMENT NETWORK

The full measurement setup diagram as well as the description can be found in Fig. 1.

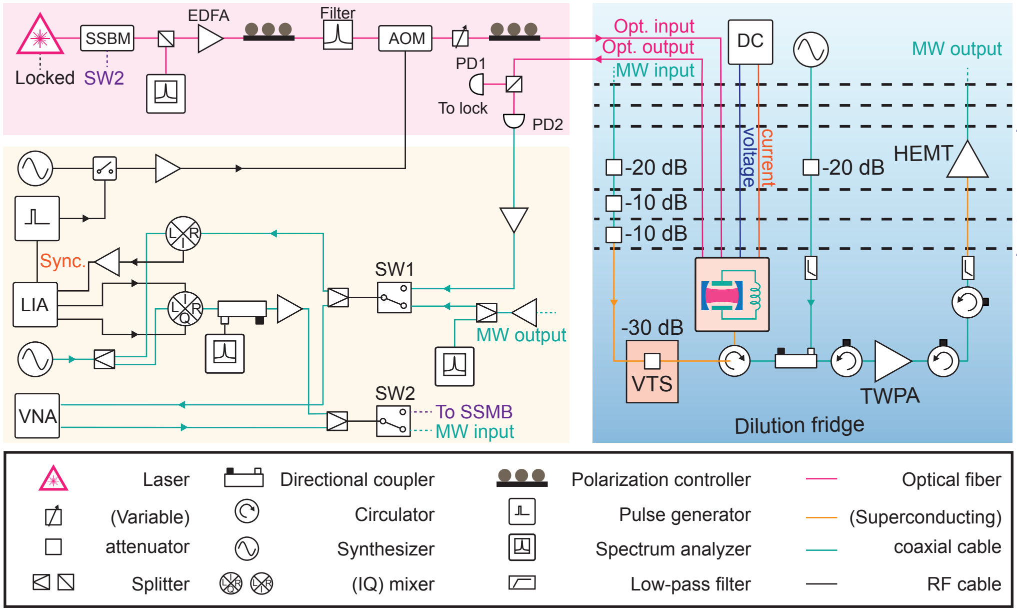


Supplementary Figure 1. Full measurement network. The whole network is divided into three sections: optical, RF, and dilution fridge sections. Signals near the microwave resonant frequency are generated by a vector network analyzer (VNA), or microwave synthesizer modulated by a Lock-in amplifier (LIA) via an IQ mixer. A switch (SW) sends the signals either to the transducer's microwave port after a chain of attenuators, or to the optical single-sideband modulator (SSBM), which up-converts the signal to the signal optical mode's frequency before being sent to the transducer's optical port. After the device, signals from the microwave output port are detected by a spectrum analyzer (SA), the VNA, and the LIA. The optical output signals are detected by two photodetectors (PDs). PD1 detects the power of the output and provides feedback to the laser. PD2 performs heterodyne detection for the optical output, where optical signal and drive beats and down-converts the signals. Inside the fridge, the transducer is installed in the MXC (40 mK). Fibers feed-through are made for optical input and readout. In the microwave line, a variable temperature stage (VTS) is employed and installed right before the transducer to calibrate the gain and added noise of the output line. The output line consists of a travelling wave parametric amplifier (TWPA) followed by a high-electron-mobility transistor (HEMT) amplifier, which provide precision measurement with added noise around 4 quanta. The circulators ensures an impedance matching environment for the TWPA. DC voltage and current are sent to the transducer to tune the optical and microwave's frequencies in situ. A microwave tone is sent through a directional coupler to the TWPA as its pump.

### A. conversion efficiency calibration

To unambiguously calibrate the conversion efficiency of our converter device, we measure spectra of the complete conversion matrix. Utilizing two microwave switches (SW1 and SW2), we measure $|S_{eo}|$, $|S_{oe}|$, $|S_{ee}|$, and $|S_{oo}|$ when applying a 4.6 dBm pulsed optical drive, as shown in Fig. 2, without changing any optical or microwave wirings. All conversion spectra are fit to Lorentzian functions as shown in the red solid curves. Following the calibration procedure

in reference [1], loss/gain in the optical and microwave input/output chains are calibrated out and the conversion efficiency is obtained, without using any additional parameters, as $2.4 \times 10^{-5}$.

To calculate conversion efficiency with weaker laser drives, we use the calibrated conversion efficiency at 4.6 dBm as a reference, and only measure $|S_{\rm eo}|$ which has a much better signal to noise ratio than $|S_{\rm oe}|$. Because the measurement system is linear, the conversion efficiency scales linearly with the peak of $|S_{\rm eo}|$. As a result, the conversion efficiency with lower optical drive can be determined.

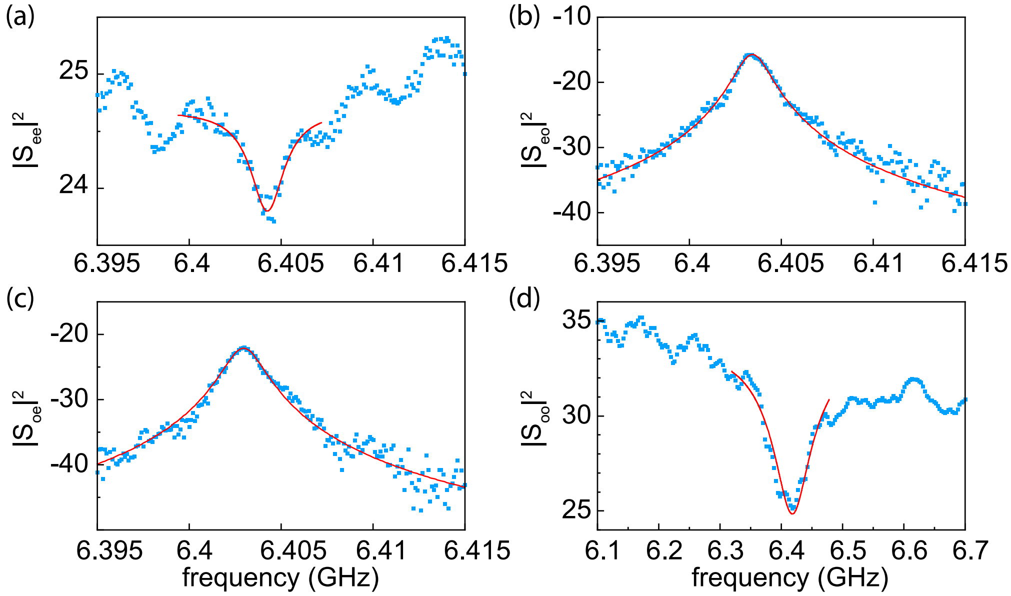


Supplementary Figure 2. Four elements of the scattering matrix for self-referencing calibration

### B. Microwave output line calibration

Output line gain and added noise calibration at microwave frequencies is essential to determining the absolute value of the light-induced noise amplitude coming from the device under test. The output line calibration is conducted by measuring a known variance in the mixing chamber of the dilution refrigerator provided by a variable temperature stage (VTS), see Fig. 1. The VTS is thermally isolated from the rest of the fridge, so its temperature can be controlled by a heater while the rest of the fridge experiences a negligible temperature change. The temperature of the VTS is monitored by a Ruthenium Oxide (RuOx) thermometer. A 30 dB attenuator is mounted on the VTS, with optimized thermal contact, to serve as the known thermal source. The variance of attenuator output satisfies Bose-Einstein distribution: $\bar{n}_{\rm vts} = 1/\big(\exp(hf/k_{\rm B}T_{\rm vts}) - 1\big)$.

First we present the model for output line calibration. When we perform output line calibration, the microwave resonance is detuned from frequencies of interest, so the device can be regarded as a perfect reflector. The measured symmetrical noise power spectral density $\bar{S}_{\rm out}$ is thus linked to the VTS output through:

$$\bar{S}_{\rm out} = G_{\rm vts}(\bar{n}_{\rm vts,s} + \bar{n}_{\rm vts,i} + N_{\rm add,vts} + 1). \quad \text{(S3)}$$

Here $\bar{n}_{\rm vts,s}$ and $\bar{n}_{\rm vts,i}$ are the thermal occupancy of VTS output at the amplifier's signal and idler frequencies, respectively. $G_{\rm vts}$ and $N_{\rm add,vts}$ are the gain and extra thermal noise of the entire output chain with respect to the VTS. The last term 1 in the bracket represents the quantum noise. Note that here we assume the gain of the parametric amplifier is very large otherwise the gain coefficient for $\bar{n}_{\rm vts,s}$ and transduction coefficient for $\bar{n}_{\rm vts,i}$ will be different. Another assumption we make is that the attenuation between the VTS and the TWPA is the same for the signal and the idler frequencies. Compared to our previous work using a Josephson parametric converter as the pre-amplifier, the calibration model is slightly different because we have to take into account the VTS noise at the idler frequency [2]. It is because for JPC, the idler mode input is separate from the signal mode input, while for TWPA, there is only one port for both signal and idler inputs.

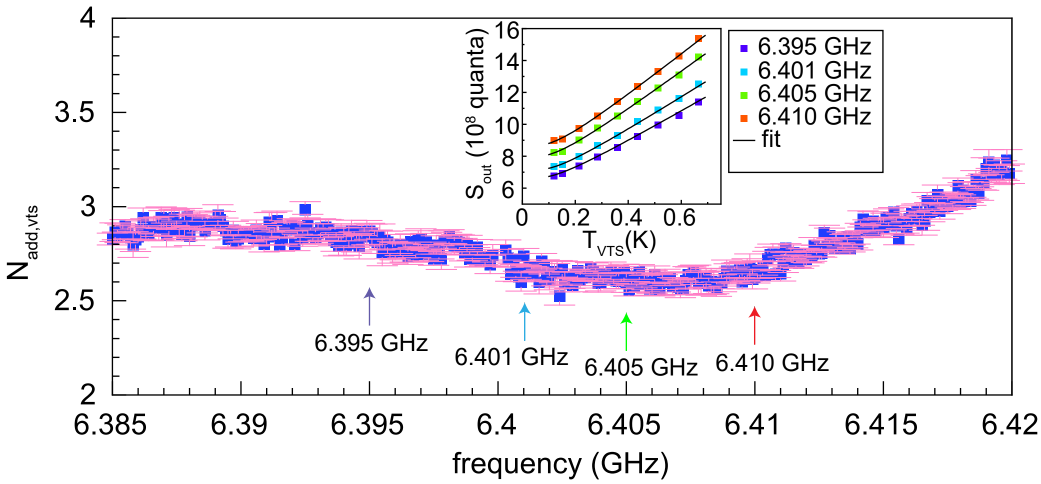


Supplementary Figure 3. The results of $N_{\mathrm{add,vts}}$ as a function of frequency. Shown in the inset are symmetrical noise spectra $\bar{S}_{\mathrm{out}}$ as a function of VTS temperature. Each curve corresponds to a different frequency. The solid curve shows fit to the theory which reveals the added noise $N_{\mathrm{add,vts}}$ and gain $G_{\mathrm{vts}}$ of the output line. The typical output line gain of frequencies of interest is around $G_{\mathrm{vts}}$ =83 dB.

To perform the output line calibration, we heat up the VTS to elevated temperatures up to 660 mK. When thermal equilibrium is reached at each temperature, we measure the symmetrical noise power spectral density $\bar{S}_{\mathrm{out}}(\omega)$ using a spectrum analyzer at the end of the output chain. Then we plot the $\bar{S}_{\mathrm{out}}$ at each frequency against the VTS temperature (see the inset of Fig. 3), and fit the curve to eq. S3. The gain $G$ and added noise $N_{\mathrm{add,vts}}$ can be thereby determined. Fig. 3 shows that the total added noise of the output chain is around $N_{\mathrm{add,vts}}+1=4$ quanta. Given the calibrated gain results, the attenuation of the input line can also be determined by characterizing the transmission from the room temperature input line to the output line with a vector network analyzer.

The above discussion shows the calibration of the output line with respect to the VTS, while to determine the absolute noise from the device, we need the gain ($G_{\mathrm{dev}}$) and added noie ($N_{\mathrm{add,dev}}$) with respect to the device. Because of the small attenuation ($L$) between the VTS and the device, which is mainly due to the loss in the circulator (see Fig. 1), the $G_{\mathrm{dev}}$ is slightly larger than $G_{\mathrm{vts}}$: $G_{\mathrm{dev}} = G_{\mathrm{vts}}/L$. While for added noise, $N_{\mathrm{add,dev}}$ is slightly smaller: $N_{\mathrm{add,dev}} = LN_{\mathrm{add,vts}}$. According to our previous experiment with similar configuration, the attenuation $L = 91\%\pm4\%$. Thus $G_{\mathrm{vts}}$ can be used as a good estimation of $G_{\mathrm{dev}}$ to the accuracy of 10%. Because of this systematic error, the characterized device noise presented in the work should be slightly larger than the actual device noise.

When characterizing the device output noise, we operates with different TWPA gains. By assuming that the input line attenuation remains the same, we can constantly monitor the output line gain from the device by measuring the total transmission using VNA.

## NOTE 4. SUPERCONDUCTING RESONANCE UNDER OPTICAL DRIVE

When an optical drive is applied to the transducer device, the changes of the superconducting microwave resonance are mainly attributed to two reasons: ambient temperature increase and optical photon absorption by superconductor. The ambient temperature rises mainly because of the optical absorption heating of the dielectrics. The temperature change has two effects on the superconducting resonator. On the one hand, the two level systems (TLS), which are embedded in the substrate and couples to the superconducting resonator, become thermally excited at higher temperatures. This results in improved microwave intrinsic Q and increases resonant frequency [3–5]. On the other hand, the increase of temperature gives rise to increased kinetic inductance [6], which results in lower resonant frequencies. In additional to the ambient temperature change, quasi-particles are generated in the superconductor because of superconductor absorption of optical photons. This effect result in more loss to the resonance as well as down-shifted resonant frequency.

Shown in Fig. 4(a) is the device package temperature at different optical drive power. The data is obtained using a RuOx thermometer directly mounted on the package of the electro-optical device. Because of the temperature gradient, the temperature of the mixing chamber monitored by a thermometer mounted on another plate of the mixing chamber only sees 20 mK temperature increase from 44 mK at the highest optical drive shown in Fig. 4(a). Also because of the gradient, the ambient temperature of the microwave resonance is supposed to be even higher

than the results in Fig. 4(a). This result shows that the device package heating only rely on the average power of the optical drive.

Microwave resonance properties, including the frequency and intrinsic Q are plotted in Fig. 4 (b) and (c). The microwave resonant frequency first slightly increases and then decrease, and the intrinsic Qs have similar trend. Similar behavior was also observed in superconducting resonators at cryogenic temperatures in previous work [3, 5]. The increase of resonant frequency and intrinsic Q are typically attributed to the saturation of TLS while the downturn of resonant frequency and intrinsic Q are attributed to temperature-dependent kinetic inductance as well as quasi-particles generation. When a weak CW drive is applied, it appears the saturation of TLS plays a much more important role so that the frequency and intrinsic Q both increase. When switching from a CW drive to a pulsed drive. Because of the significantly less average heating power as well as the stronger peak optical power, the quasi-particles generation due to superconductor absorption of optical photons is the leading factor that affects the superconducting resonator. We observed a drastic resonant frequency drop as well as a decrease in the intrinsic Q.

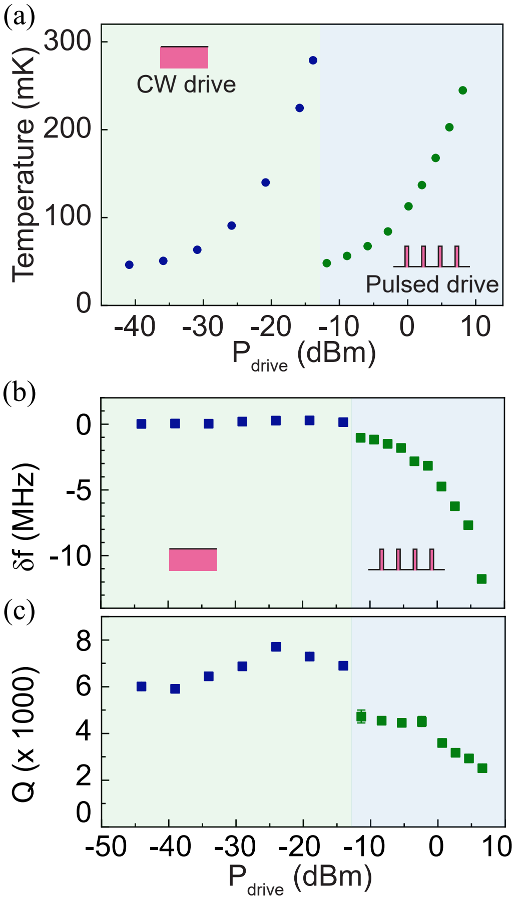


Supplementary Figure 4. Device packaging temperature (a), microwave frequency shift (b), and microwave Q (c) at different optical drive power.

## NOTE 5. TELEPORTATION FIDELITY

The cavity electro-optic platform is suitable for teleportation-based transduction [7]. By pumping the higher frequency optical mode ($b$), the output of the microwave-optical modes will be prepared in an entangled two-mode Gaussian state, which could be used as a resource in the well-knonw Braunstein-Kimble teleportation setup, realizing bidirectional quantum state transfer [8, 9]. For instance, Alice and Bob hold the two output modes $a$ and $c$, respectively, and the input state they want to transfer. A local EPR measurement on either side will enable the recovery of the input state on the other side given the measurement result is shared. The performance of this protocol can be quantified by teleportation fidelity $F$, which is the average overlap between the input state and the teleported output state. For pure single mode Gaussian state as input, the fidelity can be expressed as [10]

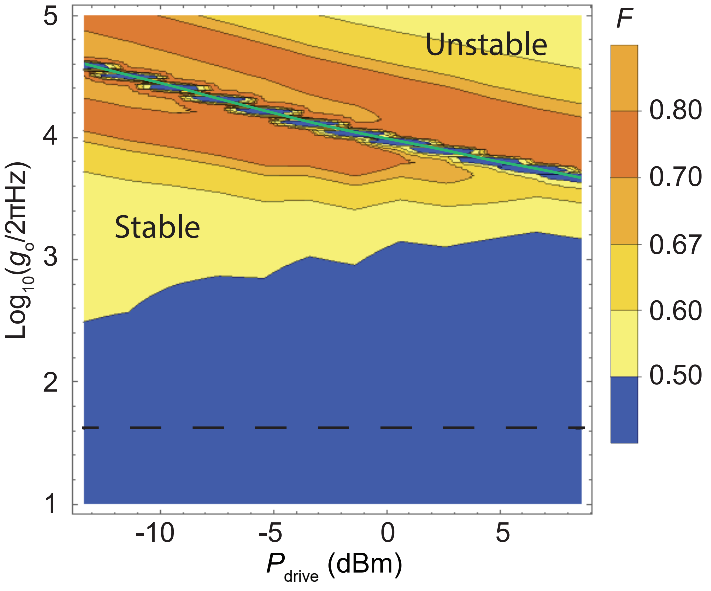


Supplementary Figure 5. Teleportation fidelity $F$ of a single mode coherent input as a function of the optical drive power $P_{\rm drive}$ and the vacuum electro-optical coupling strength $g_{\rm o}$. The extraction ratios on the optical and microwave side are taken to be 80% and 90%, respectively, corresponding to overcoupled condition. Other parameters including the microwave and optical mode intrinsic loss, optical cavity photon number and microwave intrinsic bath noise under different optical drive powers are experimental values. Notice the contour line is not smooth since the experiment data error bar is not considered in the plot. The green line separates the stable (below) from the unstable (above) regimes.

$$F = \frac{2}{\sqrt{\mathrm{Det}\left[2\mathbf{V}_{\rm in} + \mathbf{ZAZ} + \mathbf{B} - \mathbf{ZC} - (\mathbf{ZC})^{\rm T}\right]}}, \tag{S4}$$

where $\mathbf{Z} = \mathrm{diag}(1, -1)$ and $\mathbf{V}_{\rm in}$ denotes the covariance matrix of the input mode. The $2 \times 2$ real matrix blocks $\mathbf{A}$, $\mathbf{B}$ and $\mathbf{C}$ form the covariance matrix of the entangled two-mode Gaussian state

$$\mathbf{V} = \begin{pmatrix} \mathbf{A} & \mathbf{C} \\ \mathbf{C}^{\rm T} & \mathbf{B} \end{pmatrix}. \tag{S5}$$

For the teleportation protocol to be truely quantum, the fidelity must surpass a certain threshold. In this paper, we take the coherence state as the single mode input, and adopt the "no-cloning threshol" $F_{\rm th} = 2/3$ [11] as a criteria for the teleportation fidelity $F$. Here we show simulation results to provide perspectives of using cavity electro-optical system for continuous variable teleportation. Assuming perfect homodyne measurement, we compute the teleportation fidelity of a coherent state as the input using Eq. S4 based on our current device parameters. In the simulation, We use experimental values including microwave intrinsic bath occupancy, microwave intrinsic loss rate, optical intrinsic loss rate and optical cavity photons at different optical drive powers. We assume that we can optimize the external coupling rates for the optical mode and the microwave mode to have extraction ratios $\frac{\kappa_{\rm a,ex}}{\kappa_{\rm a}} = 80\%$ and $\frac{\kappa_{\rm c,ex}}{\kappa_{\rm c}} = 90\%$, respectively. The electro-optical coupling $g_{\rm o}/2\pi$ is swept from 10 Hz to $10^5$ Hz. Fig. 5 plots the teleportation fidelity $F$ as a function of the optical pump power and the electrical-optical coupling strength $g_{\rm o}/2\pi$. Our current experimental $g_{\rm o}/2\pi$ is marked as the dashed line. With our current device configuration, achieving a teleportation fidelity over this threshold still remains elusive. It is mainly because of the relatively weak vacuum electro-optical coupling rate $g_{\rm o}$. In the main text we have discussed the reasons for weak $g_{\rm o}$ and potential approaches to improve $g_{\rm o}$. The fidelity could be larger than the "no-cloning threshol" when $g_{\rm o}/2\pi$ is improved to 4000 Hz by pumping with a -2 dBm optical drive, which is promising to reach given the fast development of electro-optic platform.

[1] L. Fan, C.-L. Zou, R. Cheng, X. Guo, X. Han, Z. Gong, S. Wang, and H. X. Tang, Science Advances.

[2] M. Xu, X. Han, C.-L. Zou, W. Fu, Y. Xu, C. Zhong, L. Jiang, and H. X. Tang, Phys. Rev. Lett. **124**, 033602 (2020).
[3] D. Niepce, J. Burnett, and J. Bylander, Phys. Rev. Applied **11**, 044014 (2019).
[4] T. Lindström, J. E. Healey, M. S. Colclough, C. M. Muirhead, and A. Y. Tzalenchuk, Phys. Rev. B **80**, 132501 (2009).
[5] J. Gao, M. Daal, A. Vayonakis, S. Kumar, J. Zmuidzinas, B. Sadoulet, B. A. Mazin, P. K. Day, and H. G. Leduc, Applied Physics Letters **92**, 152505 (2008), https://doi.org/10.1063/1.2906373.
[6] A. J. Annunziata, D. F. Santavicca, L. Frunzio, G. Catelani, M. J. Rooks, A. Frydman, and D. E. Prober, Nanotechnology **21**, 445202 (2010).
[7] A. Rueda, W. Hease, S. Barzanjeh, and J. M. Fink, npj Quantum Information **5**, 1 (2019).
[8] S. L. Braunstein and H. J. Kimble, Phys. Rev. Lett. **80**, 869 (1998).
[9] S. Barzanjeh, M. Abdi, G. J. Milburn, P. Tombesi, and D. Vitali, Phys. Rev. Lett. **109**, 130503 (2012).
[10] C. Weedbrook, S. Pirandola, R. García-Patrón, N. J. Cerf, T. C. Ralph, J. H. Shapiro, and S. Lloyd, Rev. Mod. Phys. **84**, 621 (2012).
[11] F. Grosshans and P. Grangier, Phys. Rev. A **64**, 010301 (2001).
